# Supplementary material for: Mining Word Boundaries from Speech-Text Parallel Data for Cross-domain Chinese Word Segmentation
Source: arXiv:2412.09045 source file (2024-12-12)
Supplement: Supplementary file 1 [file 9-appendix.tex]

\appendix

\section{Annotation of AISHELL-dev/test}
