# Supplementary material for: Mining Word Boundaries from Speech-Text Parallel Data for Cross-domain Chinese Word Segmentation
Source: arXiv:2412.09045 source file (2024-12-12)
Supplement: Supplementary file 2 [file 9.2-appendix.tex]

\section{Marginal Probability}

% 将分词看作序列标注问题（bmes），
% 输入序列x，标签序列y，
% 那么一个序列的分数为：s(x,y) = sum(s(x-i))， i属于y
% 在CRF中，条件概率p(y|x) = e^s(x,y) / Z(x)=所有分数之和
% loss = -s(x,y) + logZ
% 一个位置某个标签的边缘概率
% p(l|x) = 

For CWS, we approach it as a sequence labeling task using the label set $\{B, M, E, S\}$.
Given an input sequence {$\boldsymbol{x}={x_0, ..., x_n}$}, a possible label sequence is {$\boldsymbol{y}={y_0, ..., y_n}$}. The score of {$\boldsymbol{y}$} is determined by summing up the scores of labels it contains.
\begin{equation}
s({\boldsymbol{x},\boldsymbol{y}) = \sum\limits_{\tiny{\boldsymbol{y}_i \in 
\boldsymbol{y}}}s(\boldsymbol{y}_i)}
\label{formula:score}
\end{equation}
In the space of all possible solutions $Y(x)$, the conditional probability under CRF is

$$
 p(y|x)=\frac{e^{s(x,y)}}{Z(x) \equiv \sum\limits_{\tiny{y^{\prime}\in Y(x)}}e^{s(x,y^{\prime})}}
$$
where $Z(x)$ is the normalization term.
The CRF loss is to maximize the conditional probability.
$$
\mathcal{\ell}(x,y)=-\log p(y|x)=\log Z(x) - s(x,y)
$$
During the inference, we can obtain the marginal probability by calculating the derivative with respect to $\log Z(x)$. 
$$
p(y_i|x)=\frac{\partial{\log Z(x)}}{\partial{s(y_i)}}
$$
The probability of a word boundary is determined by summing the probabilities of labels 'E' and 'S'.
